# Supplementary material for: SphNet: A Spherical Network for Semantic Pointcloud Segmentation
Source: arXiv:2210.13992 source file (2022-10-24)
Supplement: Supplementary file 1 [file supp_qualitative.tex]

\section{Additional Qualitative Results}
In this section, we initially further discuss the qualitative results of our proposed semantic segmentation framework.
Next, we state additional improvements that can be made and elaborate on the limitations of the proposed spherical multi-modal segmentation framework. 

All predictions in this section are based on a spherical bandwidth of $100$ and $150$ for pointclouds and images, respectively. 

\subsection{Spherical Semantic Segmentation}\label{sec:supp:sph}
We first show the spherical semantic segmentation with respect to the spherical ground truth in Figure~\ref{figs:supp:semantic_spheres}. 
The segmentation results are achieved by additionally applying a softmax function to the logits output of our network.
In particular, the presented semantic segmentation corresponds to the output of our proposed fusion network after inferring a prior segmentation using our base network.

\begin{figure*}[!thb]
  \centering
   \includegraphics[width=0.9\textwidth, trim={0.0cm, 0.0cm, 0.0cm, 0cm}, clip]{img/Supp_Semantic_Spheres.pdf}
   \caption{Qualitative comparison of the semantic segmentation of spheres with respect to the ground truth.}
   \label{figs:supp:semantic_spheres}
\end{figure*}

In this comparison, we trained the model on the nuScenes~\cite{Caesar2020} training set and tested it on the nuScenes~\cite{Caesar2020} validation set. 
It can be noted that our semantic segmentation framework provides a reasonable good and accurate segmentation of the sampled sphere in comparison with the ground truth segmentation, even for structures and objects that are further away from the sensor.

\subsection{Back-Projected Semantic Segmentation}
Next, we show, in addition, the reprojected the pointclouds to understand better the applicability of our proposed framework in real-world scenarios.
Thus, we back-project the semantic predictions from $S^2$ to $\mathbb{R}^3$ using the initially sampled range values.
Figure~\ref{figs:supp:semantic_clouds} shows the resulting back-projected semantic segmentation results in comparison to the ground truth segmentation.

\begin{figure*}[!htb]
  \centering
   \includegraphics[width=0.9\textwidth, trim={0.0cm, 0.0cm, 0.0cm, 0cm}, clip]{img/Supp_Semantic_Clouds.pdf}
   \caption{Qualitative comparison of the semantic segmentation of the reprojected pointclouds with respect to the ground truth.}
   \label{figs:supp:semantic_clouds}
\end{figure*}

Here, we used the same training and inference setup described in Section~\ref{sec:supp:sph}.
Even in cluttered scenes, as in Figure~\ref{figs:supp:semantic_clouds} (middle), our segmentation framework provides a good segmentation of the environment. 

\subsection{Limitations and Improvements}

Although yielding promising results regarding the inference of homogeneous and heterogeneous sensor data, our approach still has certain limitations. 

Specifically, Figure~\ref{figs:supp:semantic_spheres} illustrates that the fine structure of objects and vehicles is challenging to segment for our algorithm and hence, suggests the need of a higher resolution, i.e., larger spherical bandwidth not only as input but also for the layers in-between.
However, a larger bandwidth at the layers comes at the cost of substantially higher memory requirements requiring a carefully chosen trade-off when deploying on robots.

Additionally, we provide a more detailed comparison of the semantic segmentation is given in Figure~\ref{figs:supp:details}.

\begin{figure*}[!htb]
  \centering
   \includegraphics[width=0.6\textwidth, trim={0.0cm, 0.0cm, 0.0cm, 0cm}, clip]{img/Supp_Details.pdf}
   \caption{Detailed comparison of the predicted and the ground truth segmentation. The marked area denote areas where the prediction failed to fully segment the vehicles.}
   \label{figs:supp:details}
\end{figure*}

It can be stated that upon closer examination of the semantic segmentation, some objects are not entirely encoded with the same semantic label, e.g., vehicles being partially segmented as objects. 
A potential solution to overcome this issue as well as binning artifacts from the projection (i.e., points that fall in the same equiangular grid), a kNN-based search can be used as a post-processing step~\cite{Milioto2019a}.

\paragraph{}
Finally, the generalization to the SemanticKITTI~\cite{Behley2019} underlies certain limitations. 
Figure~\ref{figs:supp:kitti} shows an inference of a pointcloud on the SemanticKITTI dataset with respect to the ground truth.

\begin{figure*}[!htb]
  \centering
   \includegraphics[width=0.7\textwidth, trim={0.0cm, 0.0cm, 0.0cm, 0cm}, clip]{img/Supp_KITTI.pdf}
   \caption{Qualitative comparison of the prediction on the SemanticKITTI~\cite{Behley2019} dataset using the model that was trained on the nuScenes~\cite{Caesar2020} dataset.}
   \label{figs:supp:kitti}
\end{figure*}

It is evident that the substantially different intensity values on the SemanticKITTI~\cite{Behley2019} has severe effects on the prediction. 
Specifically, the prediction fails to distinguish detailed structure due to the different nature of the intensity channel. 
Additionally integrating different sensor data with different resolutions during the training is a potential solution which our proposed approach seamlessly supports.
