# Supplementary material for: SphNet: A Spherical Network for Semantic Pointcloud Segmentation
Source: arXiv:2210.13992 source file (2022-10-24)
Supplement: Supplementary file 2 [file supp_code.tex]

\section{Source Code}
This section gives an overview of the provided source code that is part of this supplementary material. 
Generally, we intend to fully release the source code of our proposed framework upon publication for the benefit of the community.

The provided source code example in this supplementary material provides insights into our framework by featuring the code for the feature generation, training, and inference. 
We also provide the code for performing the pooling and unpooling operation of signals in $SO(3)$. 

All the details of the source code can be found in the enclosed \textit{README.md}.
